# Supplementary material for: Federated Learning with Heterogeneous Architectures using Graph HyperNetworks
Source: arXiv:2201.08459 source file (2022-01-20)
Supplement: Supplementary file 1 [file supp.tex]

\documentclass{article}

\usepackage{neurips_2021}

\usepackage[utf8]{inputenc} %
\usepackage[T1]{fontenc}    %
\usepackage{hyperref}       %
\usepackage{url}            %
\usepackage{booktabs}       %
\usepackage{amsfonts}       %
\usepackage{nicefrac}       %
\usepackage{microtype}      %
\usepackage{xcolor}         %
\usepackage{wrapfig}
\usepackage{floatrow}

\definecolor{myred}{rgb}{0.658, 0.188, 0.000}

\usepackage{booktabs}
\usepackage{graphicx}
\usepackage{epsfig}
\usepackage{multirow}
\usepackage[ruled,vlined]{algorithm2e}
\usepackage{amsmath}

\title{Supplementary material for: Architecture Agnostic Federated Learning using Graph HyperNetworks}

\author{Or Litany \\
  NVIDIA\\
  Pittsburgh, PA 15213 \\
  \texttt{hippo@cs.cranberry-lemon.edu} \\
}

\begin{document}

\maketitle

\appendix
\input{sections/99_supp}

\bibliography{egbib}
\bibliographystyle{abbrv}

\end{document}
